# Supplementary material for: Controlled Floquet Dynamics and Topological Bound States in Continuum via Colored Quantum Random Walks
Source: arXiv:2503.17263 source file (2025-03-21)
Supplement: Supplementary file 1 [file SM.tex]

\begin{widetext}
  \subsection*{Supplemental Material: Controlled Floquet Dynamics and Topological Bound States in Continuum via Colored Quantum Random Walks}  

\begin{quote}
\centering
    \normalsize Zahra Jalali-Mola$^1$ , Ortwin Hess$^{1,2}$\\
    $^1$\normalsize\small\textit{School of Physics and CRANN Institute, Trinity College Dublin, University of Dublin, Dublin 2, D02 PN40, Ireland}\\
$^2$\normalsize\small\textit{AMBER, SFI Research Centre for Advanced Materials and BioEngineering Research, Trinity College Dublin, University of Dublin, Dublin 2, D02 PN40, Ireland}
\\
\end{quote}

\section*{Finite structure}
  To further investigate the physical characteristics of the BICs, we switch from a semi-finite structure to a fully finite one in the $xy$-plane by considering a finite configuration of two media, where one medium is enclosed by the other.
  The energy spectrum for this configuration is illustrated in Fig.~S1(a), in which the same rotation parameters for inner and outer media as Fig.~\ref{fig:edge_STT}(a) are assumed. 
  The finite lattice size used in the analysis is $L_x=L_y=30$, with the inner medium located at the center and having a size of $l_x=l_y=10$.
  The green diamonds and the red star represent the localized edge states in the gap and BICs, respectively.
  
  In panels~(b) to~(e) we have plotted the wave function for each group of the eigenstates. The state index from the top left to the bottom right is $2,865,1854,2697$. The chiral edge states defined in green, panels~(b),~(d), and ~(e), remain localized at the edge of system, while the TBICs which were localized states at the edge, turn to the corner sates (shown in panel~(c)).
  The localization properties of the TBICs~(red star) indicate its state is localized in the corner of the boundary, similar to the higher-order topological corner states surrounded by bulk states.

  %To further explore the physical properties of the BICs, we transition from a semi-infinite structure to a fully finite one confined within the $xy$-plane. This configuration consists of two media, with one medium entirely enclosed by the other. The energy spectrum for this setup is depicted in Fig.\ref{fig:BIC}(a), where the rotation parameters for the inner and outer media are identical to those in Fig.\ref{fig:edge_STT}(a). For the finite lattice, the dimensions used are $L_x = L_y = 30$, with the inner medium positioned at the center and having a size of $l_x = l_y = 10$.
  %Localized edge states within the gap and BICs are denoted by yellow diamonds and a red star, respectively. 
 % Panels (b) to (e) illustrate the wave functions corresponding to specific eigenstates, indexed as $2, 865, 1854, 2697$ from the top left to the bottom right. Chiral edge states, indicated in blue, remain localized along the system's edges. Meanwhile, the BICs, which were previously localized along the edges in the semi-finite configuration, transition into corner states in the fully finite structure. The localization characteristics of the BIC (red star) reveal that this state is confined to the system's corners, akin to higher-order topological corner states. Notably, in some instances, edge states overlap with bulk states but retain their localized nature within the bulk.

\begin{figure}[h]
    \centering
    \includegraphics[width=0.55\linewidth]{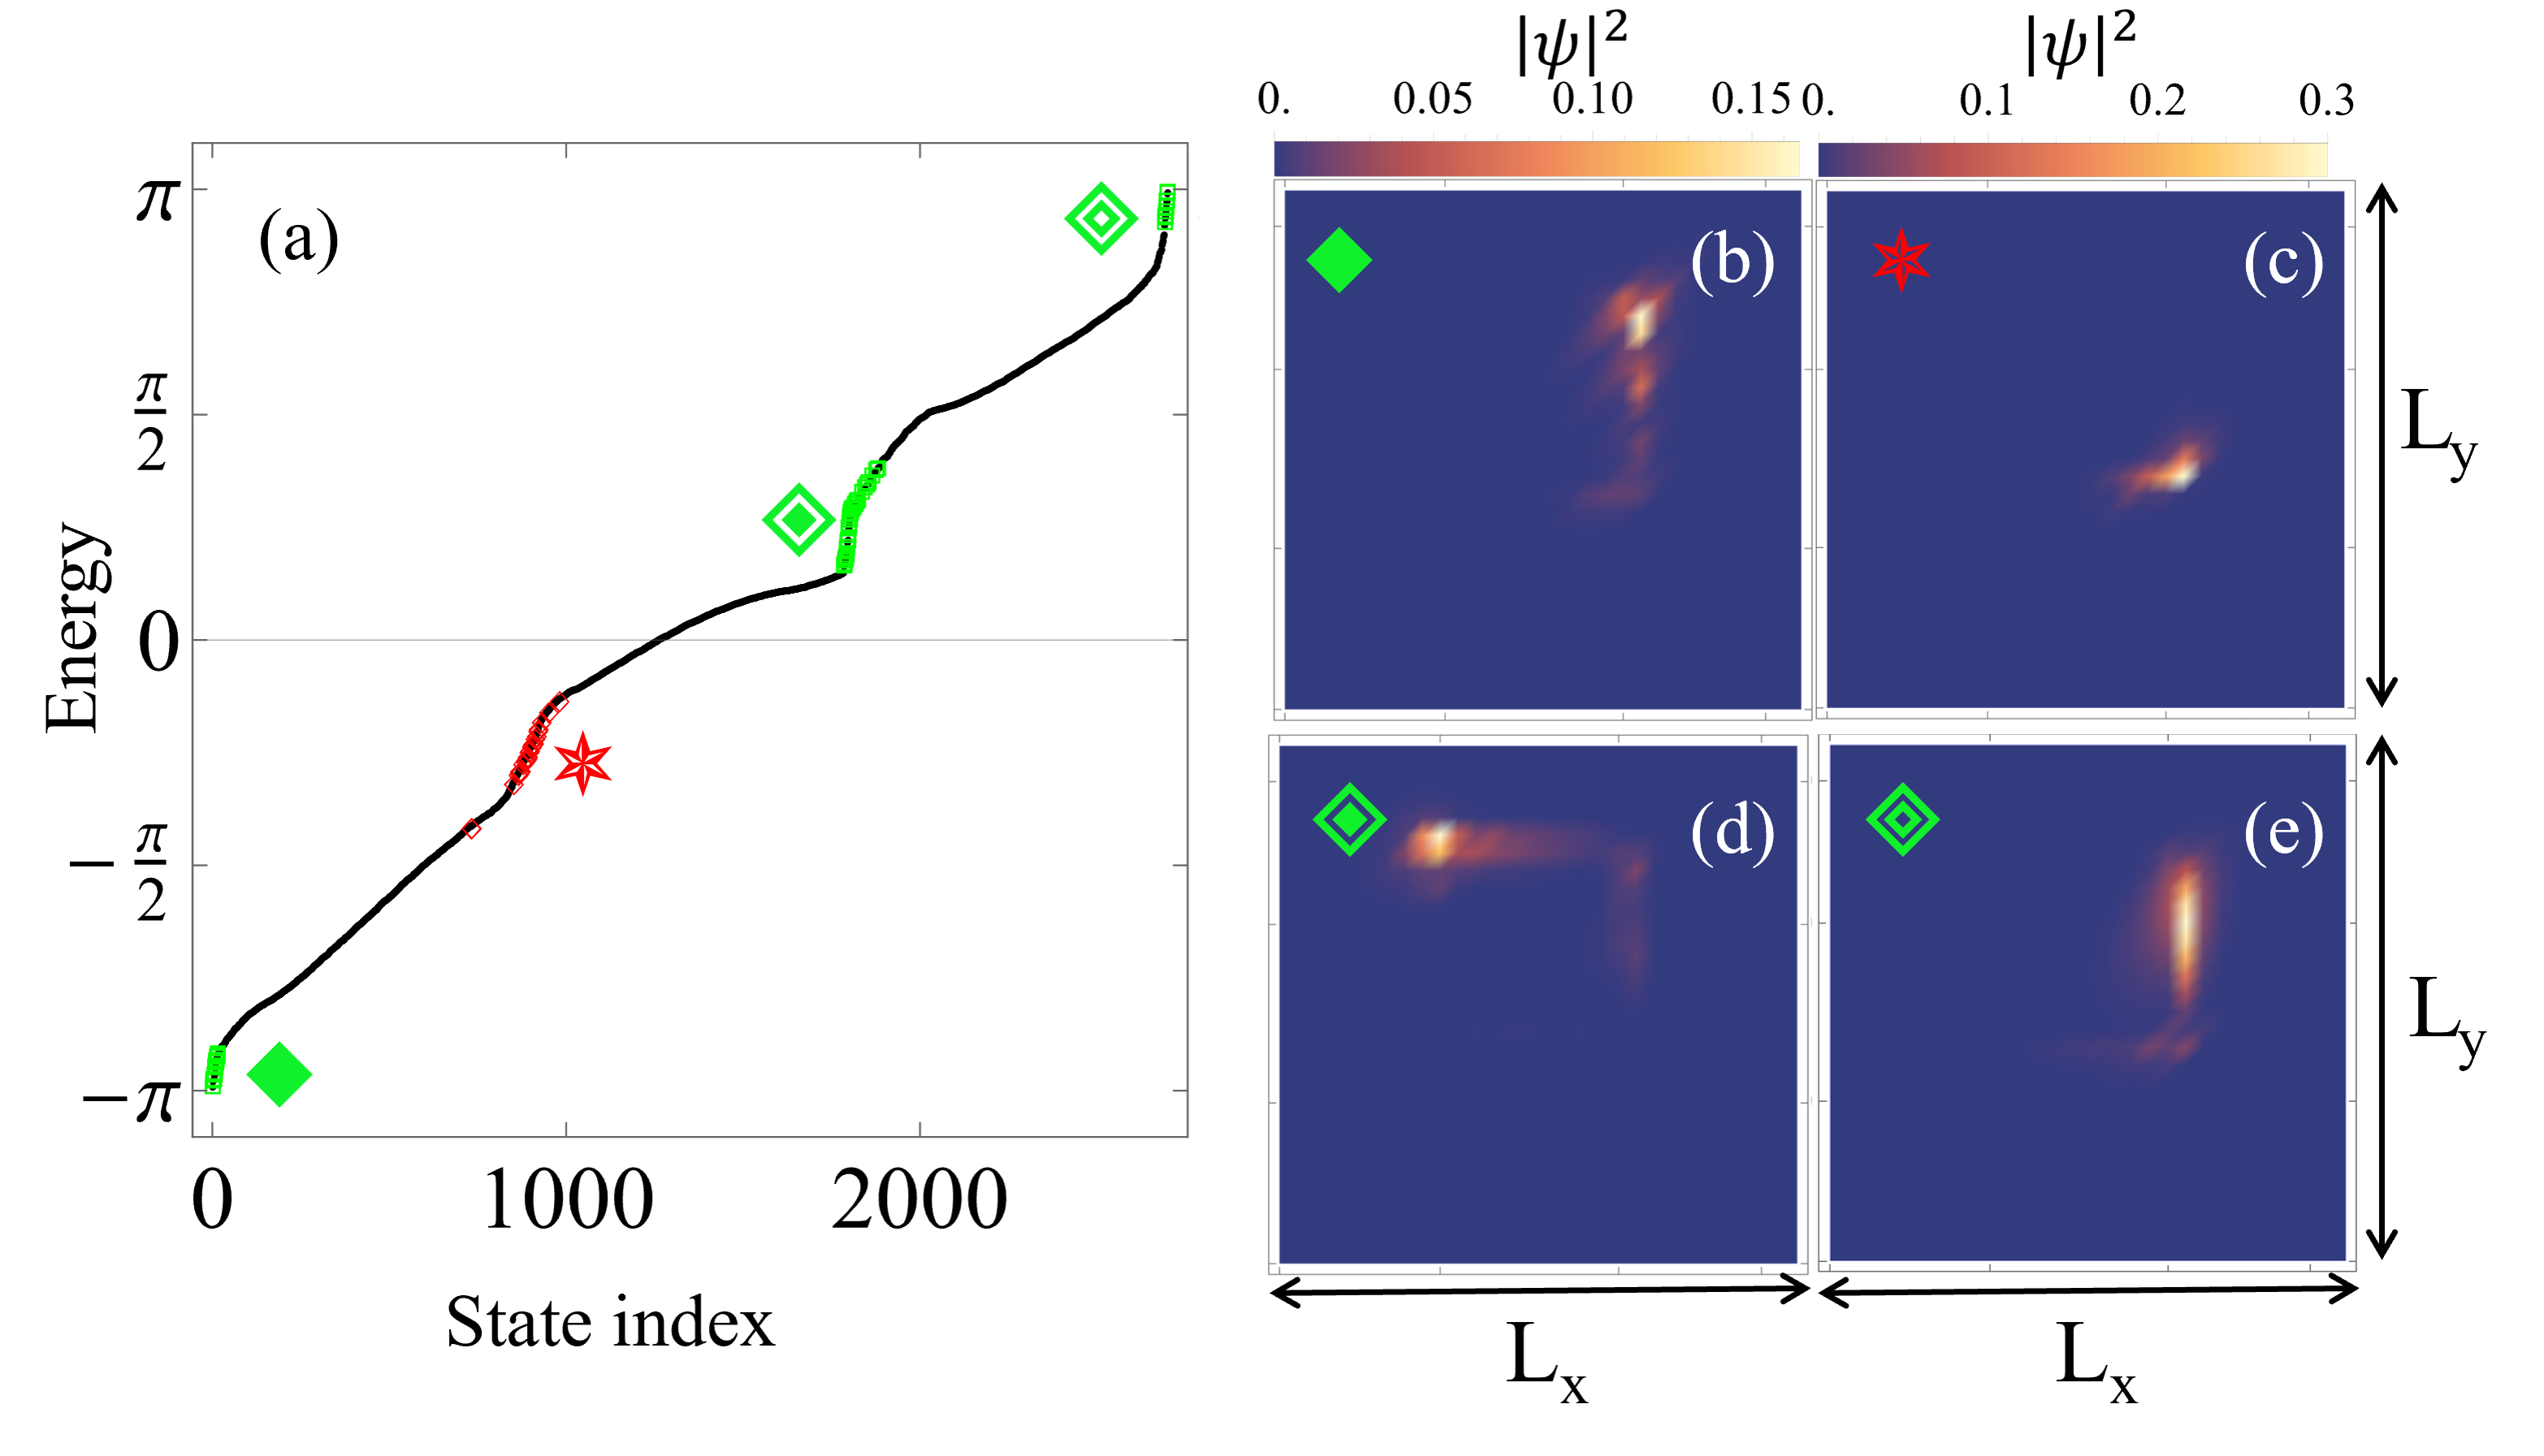}
    \caption{
    The left panel presents the energy spectrum of a finite structure confined within the $xy$-plane, while the right panel display the corresponding wave functions. This structure comprises an inner medium characterized by rotation parameters $(\theta_{1i}, \theta_{2i}) = (\pi/3, -\pi)$, enclosed by an outer medium with parameters $(\theta_{1o}, \theta_{2o}) = (-2\pi, 3\pi)$, similar to those in Fig.~\ref{fig:edge_STT}(a). The localized edge states are marked with green diamonds, and TBICs are indicated by red diamonds. The corresponding wave functions of each sector, $|\psi(x,y)|^2$, are depicted in the right panels.
    }
    \label{fig:BIC_Finite}
\end{figure}

\end{widetext}
